# Supplementary material for: Analogical Reasoning for Visually Grounded Language Acquisition
Source: arXiv:2007.11668 source file (2020-07-22)
Supplement: Supplementary file 1 [file appendix.tex]

\section{Appendix}

\paragraph{Implementation Details [XX: move to Appendix?]}
In all experiments, training is conducted on 2 GPUs for 200 epochs. In each mini-batch, 256 samples are drawn for each GPU and in each sample, image regions are cropped from the whole image and resized to $112 \times 112$. The transformer encoder in all models has the same configuration: 4 layers, a hidden size of 384, and 4 self-attention heads in each layer. 
 % And the loss weight for $L_l$ and $L_v$ are 1 and 30 respectively. 
 % BQ related
Besides, we use AdamW optimizer ~\cite{loshchilov2017decoupled} with the learning rate 3e-5. For AdamW optimizer ~\cite{loshchilov2017decoupled}, we set the update coefficients, for averages of gradient and its square ($\beta_1$, $\beta_2$), and $\epsilon$ on denominator as 0.9, 0.999, 1e-4.
During training, we mask out text tokens $\frac{1}{3}$ of the time and image tokens $\frac{1}{6}$ of the time and follow the same setting of random masking strategy with BERT ~\cite{devlin2018bert}. 
% Following BERT ~\cite{devlin2018bert}, a masked text token gets assigned a special [MASK] token $80\%$ of the time, a random word token $10\%$, and remains unchanged $10\%$. Similarly, we zero out image tokens $90\%$ of the time and leave them unaltered $10\%$. 
During training and testing, for each target sample, we randomly select 200 remaining samples as the corresponding reference set. In our experiments, we utilize Top-K (K = 3) reference samples to get involved in analogical reasoning.

% As shown in Figure~\ref{fig:tar_ref_vis}, the model can successfully retrieve relevant reference samples that which contain analogical pairs.
From the two examples shown in Figure~\ref{fig:tar_ref_vis}, it's easy to observe that the model can successfully retrieve relevant reference samples which contain analogical pairs, by computing their visual and language similarity to the target composition. For the correct prediction ``peel carrot'', the model discovers ``stir carrot'', ``peel potato'' and ``cut potato'' for analogical reasoning, while for ``wash knife'', the model retrieves ``wash plate'', ``take knife'' and ``rinse knife'' as reference samples.

\begin{figure}[ht]
\centering
\includegraphics[width=0.8\textwidth]{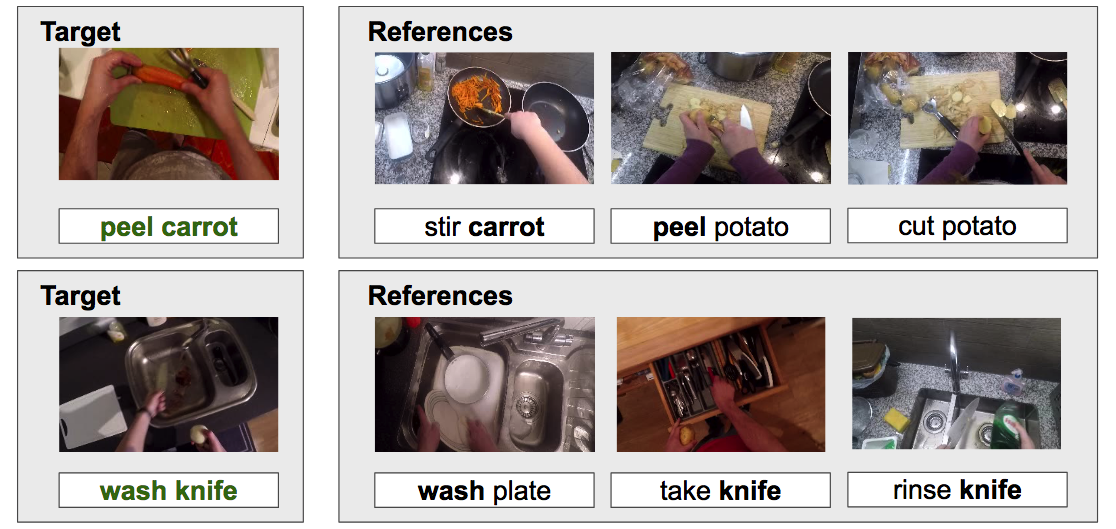}
\caption{The target sample and top samples discovered from the reference set.}
\label{fig:tar_ref_vis} 
\end{figure}
